# Supplementary material for: LaCAM: Search-Based Algorithm for Quick Multi-Agent Pathfinding
Source: arXiv:2211.13432 source file (2022-11-24)
Supplement: Supplementary file 1 [file small-complicated-appendix.tex]

{
  \setlength{\tabcolsep}{2.2pt}

  \begin{table}[th!]
  \scriptsize
    \centering
    \begin{tabular}{lrrrrrrrrrrrrc}
      \toprule
      & \multicolumn{2}{c}{\mapname{tree}}
      & \multicolumn{2}{c}{\mapname{corners}}
      & \multicolumn{2}{c}{\mapname{tunnel}}
      & \multicolumn{2}{c}{\mapname{string}}
      & \multicolumn{2}{c}{\mapname{loop-chain}}
      & \multicolumn{2}{c}{\mapname{connector}}
      \\
      \cmidrule(lr){2-3}
      \cmidrule(lr){4-5}
      \cmidrule(lr){6-7}
      \cmidrule(lr){8-9}
      \cmidrule(lr){10-11}
      \cmidrule(lr){12-13}
      \cmidrule(lr){2-3}
      \cmidrule(lr){4-5}
      \cmidrule(lr){6-7}
      \cmidrule(lr){8-9}
      \cmidrule(lr){10-11}
      \cmidrule(lr){12-13}
      & T & SOC
      & T & SOC
      & T & SOC
      & T & SOC
      & T & SOC
      & T & SOC
      & Solved
      \\
      \cmidrule{1-1}
      \cmidrule(lr){2-3}
      \cmidrule(lr){4-5}
      \cmidrule(lr){6-7}
      \cmidrule(lr){8-9}
      \cmidrule(lr){10-11}
      \cmidrule(lr){12-13}
      \cmidrule(lr){14-14}
      Bm
      & 0 & 19
      & 17 & 47
      & 173 & 190
      & 0 & 66
      & 34 & 1752
      & 0 & 168
      & \multirow{2}{*}{\textbf{6/6}}
      \\
      Bw
      & 0 & 41
      & 31 & 70
      & 208 & 254
      & 0 & 68
      & 124 & 2593
      & 3 & 281
      \\\cmidrule{1-14}
      Dm
      & 0 & 47
      & 1 & 345
      & 61 & 5098
      & 0 & 66
      & 31 & 16490
      & 0 & 168
      & \multirow{2}{*}{\textbf{6/6}}
      \\
      Dw
      & 0 & 146
      & 16 & 2278
      & 75 & 6120
      & 0 & 68
      & 179 & 70785
      & 9 & 4370
      \\\cmidrule{1-14}
      Gm
      & 0 & 23
      & 0 & 40
      & 159 & 124
      & 0 & 40
      & 306 & 1526
      & 12 & 294
      & \multirow{2}{*}{\textbf{6/6}}
      \\
      Gw
      & 0 & 36
      & 14 & 58
      & 170 & 186
      & 0 & 57
      & 952 & 3074
      & 59 & 442
      \\
      \bottomrule
    \end{tabular}
    \caption{
      \textbf{Results in small complicated instances with different LaCAM designs.}
      `B,' `D,' and `G' represent Base, DFS, and GREEDY, respectively.
      `m' and `w' represent the median and worst scores.
      `T' corresponds to runtime; the unit is milliseconds.
    }
    \label{table:small-complicated-appendix}
  \end{table}
}
